# Supplementary material for: Hypernode Automata
Source: arXiv:2305.02836 source file (2024-01-08)
Supplement: Supplementary file 1 [file proofs.tex]

%\clearpage
\section{Proofs}

\subsection{Stutter-free Automata}

The proposition below proves that stutter-free automata only accept
stutter-free unzipped traces.

\begin{proposition}
\label{prop:stut_free_aut:lang}
Let \(\stutFreeA\) be a \(\Prop\)-stutter-free automaton over a domain \(\alphabet\).
The \(\stutFreeA\)-accepted language 
\(\Lang(\stutFreeA)\) is a set of minimal unzipped traces, i.e.\ \(\Lang(\stutFreeA) \subseteq \Redux{\AllAsyncTn}\).
\end{proposition}

\begin{proof}
Consider an arbitrary stutter-free automaton \(\stutFreeAFull\). 
Assume towards a contradiction that there exists an unzipped trace in the accepted language of \(\stutFreeA\), \(\trace \in \Lang(\stutFreeA)\) that  is not stutter-free, \((\star)\ \trace \notin \Redux{\AllAsyncTn}\). As \(\trace \in \Lang(\stutFreeA)\), then there exists an accepting run \(\std_0 \ldots \std_{|\trace|}\) for \(\trace\).  From our assumption \((\star)\), there exists an index \(0 \leq i < |\trace|-1\) where a variable repeats its valuation and the value is not \(\pad\). Formally, \ \(\trace(i,x) = \trace(i+1,x)\) and \(\trace(i,x) \neq \pad\). Then, there exists the following transitions in \(\stutFreeA\): \(q_{i+1} \in \Transition(q_{i},V)\), \(q_{i+2} \in \Transition(q_{i+1},V')\) and \(V(x) = V'(x) \neq \{\pad\}\).
This contradicts our assumption that \(\stutFreeA\) is a stutter-free automaton, because then \(\Pre{q_{i+1}}{x} \cap \Pos{q_{i+1}}{x} \not\subseteq \{\pad\}\).
\end{proof}

%\begin{definition}
%\label{def:suttfree:bi_boolean_closure}
Given two stutter-free automata, \(\stutFreeA_1 = (\States_1, \SInitial_1, \SFinal_1, \alphNSFA,\Transition_1)\) and
\(\stutFreeA_2 = (\States_2, \SInitial_2,\) \(\SFinal_2,\alphNSFA,\Transition_2)\), then their \emph{union} is defined as \(\stutFreeA_1 \cup \stutFreeA_2 = (\States_1 \dot{\cup} \States_2, \SInitial_1  \dot{\cup} \SInitial_2, \SFinal_1 \dot{\cup} \SFinal_2, \alphNSFA, \Transition_{\cup})\) where \(\Transition_{\cup}(\std) = \Transition_i(\std)\) when \(\std \in \States_i\) with \(i \in \{1,2\}\);
and their \emph{intersection} as 
\(\stutFreeA_1 \cap \stutFreeA_2 = (\States_1 \times \States_2, \SInitial_{\cap}, \SFinal_{\cap},\alphNSFA, \Transition_{\cap})\) where \(\SInitial_{\cap} = \{(\std_1, \std_2)\ |\ \std_1 \in \SInitial_1 \tAnd \std_2 \in \SInitial_2 \}\),
\(\SFinal_{\cap} = \{(\std_1, \std_2)\ |\ \std_1 \in \SFinal_1 \tAnd \std_2 \in \SFinal_2 \}\) and 
\(\Transition_{\cap}((\std_1, \std_2), l) = (\std_1', \std_2')\) iff
\(\Transition_1(\std_1, l) = \std_1'\) and \(\Transition_2(\std_2, l) = \std_2'\).

The \emph{determinization of \(\Prop\)-stutter-free automata \(\stutFreeA\)} over domain \(\alphabet\) is  defined as \(\deter{\stutFreeA }= (2^\States, \SInitial, \SFinal_d, \alphNSFA, \Transition_d)\) where 
\(F_d\!=\!\{S\! \in\! 2^\States \, |\, S \cap F\! \neq\! \emptyset \}\) and  
\({\Transition_d(S, V)\!=\!\bigcup\limits_{\std \in S} \Transition(\std, V)}\) with \({V\in \alphNSFA}\).
%\end{definition}

\noindent\textbf{Proposition \ref{thm:suttfree:bi_boolean_closure}.}
\emph{Let \(\stutFreeA_1 = (\States_1, \SInitial_1, \SFinal_1,\alphNSFA,\Transition_1)\) and
\(\stutFreeA_2 = (\States_2, \SInitial_2, \SFinal_2,\alphNSFA,\Transition_2)\) be two deterministic  \(\Prop\)-stutter-free automata over \(\alphabet\).
Then, both \(\stutFreeA_1 \cup \stutFreeA_2\) and 
\(\stutFreeA_1 \cap \stutFreeA_2\) are \(\Prop\)-stutter-free automata with 
\(\Lang((\stutFreeA_1 \cup \stutFreeA_2)) = \Lang(\stutFreeA_1) \cup \Lang(\stutFreeA_2))\) and \(\Lang((\stutFreeA_1 \cap \stutFreeA_2)) = \Lang(\stutFreeA_1) \cap \Lang(\stutFreeA_2))\); and
the determinization of \(\stutFreeA_1\), \(\deter{\stutFreeA_1}\), is a deterministic \(\Prop\)-stutter-free automaton over \(\alphabet\) that accepts the same language as 
\(\stutFreeA_1\), \(\Lang(\deter{\stutFreeA_1})= \Lang(\stutFreeA_1)\).}

\begin{proof}
The first part follows from a direct translation from stutter-free automaton to NFA.
The union and disjunction does not affect the stutter-free related restrictions.

Consider an arbitrary \(\Prop\)-NSFA, \(\stutFreeA_1\).
We start by proving that \(\deter{\stutFreeA_1}\) satisfies the stutter-free condition, i.e.\ 
\(\Pre{\Transition_d}{S,x} \cap \Pos{\Transition_d}{S,x} = \emptyset\), for all its states S and variables \(x \in \Prop\).
By definition:
\[
\begin{split}
\Pre{\Transition_d}{S,x} = 
&\{ l \ | \ S \in \bigcup\limits_{\std' \in S'} \Transition(\std', x:l) \} \ \ \Leftrightarrow\\
\Pre{\Transition_d}{S,x} = 
&\{ l\ |\ \forall \std \in S\ \exists \std' \tSt \std \in \Transition(\std', x:l)\}
\end{split}
\]
Thus, \((\star)\) for all \(\std \in S\), 
\(\Pre{\Transition}{\std,x} = \Pre{\Transition}{S,x}\). 
From \(\stutFreeA_1\) being a NSFA we know that, for all \(\std \in S\), 
\(\Pre{\Transition}{\std,x} \cap \Pos{\Transition}{\std,x} = \emptyset\).
Assume towards a contradiction that there exists a value that is in both the incoming and outgoing transitions of \(S\) for a variable \(x\), i.e.\ 
\(l \in \Pre{\Transition_d}{S,x} \cap \Pos{\Transition_d}{S,x}\).
Then, by definition of \(\Pos{\Transition_d}{S,x}\),
there exists a state in \(S\), \(\std \in S\), s.t.\
\(\Transition(\std, x:l) \neq \emptyset\). This contradicts our conclusion \((\star)\).

We prove now that \(\deter{\stutFreeA_1}\) satisfies the \(\pad\)-ending requirement. By \((\star)\), it follows that if
\(\pad \in \Pre{S}{x}\) then \(\pad \in \Pre{\std}{x}\) for all \(\std \in S\). So, by \(\stutFreeA\) being a NSFA it follows that for all \(\std \in S\) we have \(\Pos{\std}{x} = \{\pad\}\). Therefore \(\Pos{S}{x} = \{\pad\}\).

Finally, \(\Lang(\deter{\stutFreeA_1})= \Lang(\stutFreeA)\).
follows directly from the same result for NFA, as the determinization is done in the same way.
\end{proof}

%\subsubsection*{Proposition \ref{prop:universal_aut}.}
%\emph{Given a set of propositional variables \(\Prop\) and a finite domain \(\alphabet\), the universal \(\Prop\)-stutter free automaton over \(\alphabet\) accepts all stutter-free \vTr\ traces on \(\Prop\) over \(\alphabet\), i.e.\ \(\Lang(\uniNSFA(\alphabet, \Prop)) = \Redux{\AllAsyncTn}\).}

\begin{proposition}
\label{prop:universal_aut}
Given a set of propositional variables \(\Prop\) and a finite domain \(\alphabet\), the universal \(\Prop\)-stutter free automaton over \(\alphabet\) accepts all stutter-free unzipped traces on \(\Prop\) over \(\alphabet\), i.e.\ \(\Lang(\uniNSFA(\alphabet, \Prop)) = \Redux{\AllAsyncTn}\).
\end{proposition}

\begin{proof}
\(\Lang(\uniNSFA(\alphabet, \Prop)) \subseteq \Redux{\AllAsyncTn}\): follows from Proposition \ref{prop:stut_free_aut:lang} and from the universal automaton being a stutter-free automaton.

\(\Lang(\uniNSFA(\alphabet, \Prop)) \supseteq \Redux{\AllAsyncTn}\): a word defines a sequence of states in the universal automaton.
\end{proof}

\subsection{Model Checking Hypernode Logic}

\noindent\textbf{Corollary \ref{thm:upper_bound_mc_hypernonde}}
\emph{Let \(\KpkeOp\) be an open Kripke structure  and \(\varphi\) a hypernode formula over the same set of propositional variables, \(\Prop\). The time complexity of model checking \(\KpkeOp \models \varphi\) is \(\mathcal{O}(2^{m.|\KpkeOp|^{{|\Prop|}}})\), with \(\Var(\varphi) = \{\traceVar_1, \ldots, \traceVar_m\}\).}

\begin{proof}
\begin{enumerate}
\item Translation of the open Kripke Structure, \(\KpkeOp = (\KStates, \Prop, \KTransition, \KSIn \subseteq \KStates, \KSOut \subseteq \KStates)\), to the stutter-free automaton, \(\stutFreeA_{\KpkeOp}\) has \(\mathcal{O}(|\KStates|^{|\Prop|})\) states.

\item Determinization of \(\stutFreeA_{\KpkeOp}\), \(\deter{\stutFreeA_{\KpkeOp}} = (\States , \SInitial, \SFinal, \alphNSFA,\Transition)\), has
\(\mathcal{O}(2^{|\KStates|^{|\Prop|}})\) states.

\item Completing the \(\deter{\stutFreeA_{\KpkeOp}}\) adds \(2^{|\Prop|}\) states and so the complete \(\deter{\stutFreeA_{\KpkeOp}}\) has \(\mathcal{O}(2^{|\KStates|^{|\Prop|}})\) states. We assume from now on that \(\deter{\stutFreeA_{\KpkeOp}}\) is complete.

\item m-Self-composition of \(\deter{\stutFreeA_{\KpkeOp}}\): 
\(\mathcal{O}(|\States|^{m}) = \mathcal{O}(2^{m.|\KStates|^{|\Prop|}})\) states.\\
\end{enumerate}

The automaton \(\filter{\varphi}{+}{\deter{\stutFreeA_{\KpkeOp}^{m}}}\),
with \(\Var(\varphi) = \{\traceVar_1, \ldots, \traceVar_m\}\), has
\(\mathcal{O}(2^{m.|\KpkeOp|^{|\Prop|}})\) states. 
\end{proof}

\noindent\textbf{Corollary
\ref{thm:upper_bound_mc_hypernonde_aut}}
\emph{Let \(\Kpke = (\KStates, \Prop, \KTransition,  \KLabel)\) be a Kripke structure, \(\ActLab\) an action labeling over \(\Kpke\)'s transitions and actions \(\Actions\), and \(\KState_0 \in \KStates\) one of \(\Kpke\)'s worlds. Let  \(\fhnaut=(\States_h, \initstd, \{0,1\}^\Prop, \Actions, \Transition_h, \SLabel)\) be a hypernode automaton. The time complexity of checking  \(\Sync{\ActLab(\Kpke, \KState_0)}\in \Lang(\fhnaut)\) is \(\mathcal{O}(|\fhnaut|.2^{|\Actions| + m.|\Kpke|^{|\Prop|}})\), with \(\Var(\varphi) = \{\traceVar_1, \ldots, \traceVar_m\}\).}

\begin{proof}
\begin{enumerate}
    \item Structure with all possible slicings of \(\Kpke\),
    \(\Slice{\ActLab(\Kpke,\KState_0)} = (\States , \SInitial, \Actions, \Transition)\), has in the worst case states for all possible combinations of actions, Kripke worlds and transitions, i.e.\ it has \(\mathcal{O}(2^{|\KStates| + |\KTransition| + |\Actions|})\) states.
    
    \item The intersection of the hypernode automata with the \(\Kpke\) slicing, \(\Intersect(\fhnaut, \ActLab(\Kpke, \KState_0))\), has a state for each node of the hypernode automaton and element of the slicing. Then, it has \(\mathcal{O}(|\States_h|.|\States|)\) sates, i.e.\ \(\mathcal{O}(|\States_h|.2^{|\KStates| + |\KTransition| + |\Actions|})\) states.\\
\end{enumerate}

The check that \(\Sync{\ActLab(\Kpke, \KState)}\in \Lang(\fhnaut)\) is reduced to the emptiness problem of \(\Intersect(\fhnaut, \ActLab(\Kpke, \KState_0))\).
Then, the running time of checking \(\Sync{\ActLab(\Kpke, \KState)}\in \Lang(\fhnaut)\) is 
\(\mathcal{O}(|\fhnaut|.2^{|\Kpke| + |\Actions|}. 2^{m.|\Kpke|^{|\Prop|}})\) i.e.\ \(\mathcal{O}(|\fhnaut|.2^{|\Actions| + m.|\Kpke|^{|\Prop|}})\), where \(m\) is the largest number of trace quantifiers in the hypernode formulas.
\end{proof}
